# Supplementary material for: Revisiting Efficient Multi-Step Nonlinearity Compensation with Machine Learning: An Experimental Demonstration
Source: arXiv:2007.10025 source file (2020-07-20)
Supplement: Supplementary file 1 [file app1.tex]

%%%%%%%%%%%%%%%%%%%%%%%%%%%%%%%%%%%%%%%%%%%%%%%%%%%%%
\section{Detailed Explanation of Something} \label{app:app1}
%%%%%%%%%%%%%%%%%%%%%%%%%%%%%%%%%%%%%%%%%%%%%%%%%%%%%
